# Supplementary material for: Epistasis and Adaptation on Fitness Landscapes
Source: arXiv:2204.13321 source file (2022-06-10)
Supplement: Supplementary file 1 [file Supplementary_Figures_V3.pdf]

**Figure S1**

Illustration of the Rough-Mount-Fuji (RMF) model. Several examples of three-locus RMF landscapes with increasing epistasis, ranging from additive (left column) to the House-of-Cards model with maximum epistasis (right column).  $\sigma_{add}$  refers to the variance in the additive effect of mutations,  $\sigma_{epi}$  refers to the epistatic variance. The reference genotype is always the genotype with the lowest fitness. Single mutation steps are indicated by blue lines, blue boxes indicate binary genotypes. The underlying additive contribution to the fitness landscapes is highlighted by gray boxes and lines. The simulation code is available as Supplementary Material.

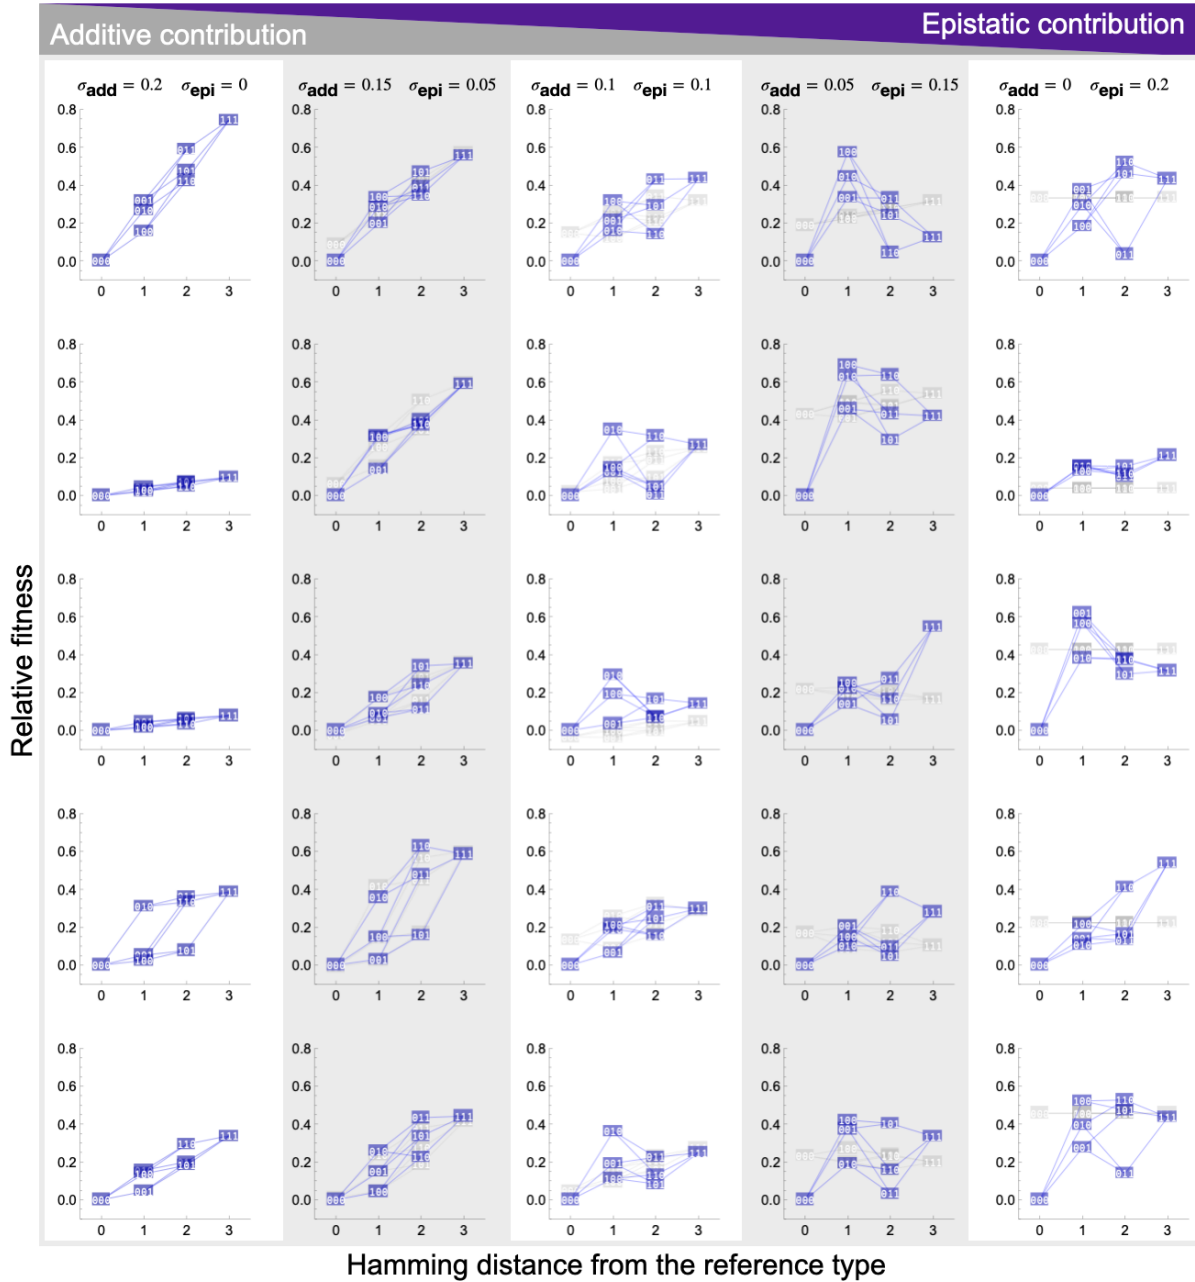

## Figure S2

Illustration of the Rough-Mount-Fuji (RMF) model and statistics of adaptive walks. (A)-(E) Evolutionary trajectories are greatly affected by epistasis. For 5 landscapes with 10 loci and increasing strength of epistasis, 1000 simulations of random adaptive walks were performed, starting at the least fit genotype in the fitness landscape. The underlying fitness landscape is drawn in gray. The evolutionary paths that were taken are drawn on the fitness landscape in blue, paths that were repeatedly taken are indicated by higher intensity. Local fitness peaks that were reached are highlighted in red, with color intensity related to the frequency of how often this endpoint was reached. The simulation code is available as Supplementary Material. In an additive fitness landscape, the single adaptive peak is reached via many different evolutionary trajectories (A). At intermediate epistasis, many of the existing adaptive peaks can be reached but evolutionary trajectories become constrained by epistasis. At maximum epistasis, few evolutionary paths remain open and only the local fitness landscape is explored by the adaptive walks (E). With increasing epistasis, the number of peaks increases and the number of unique mutational steps decreases; intermediate epistasis maximizes the divergence between evolutionary endpoints (F).

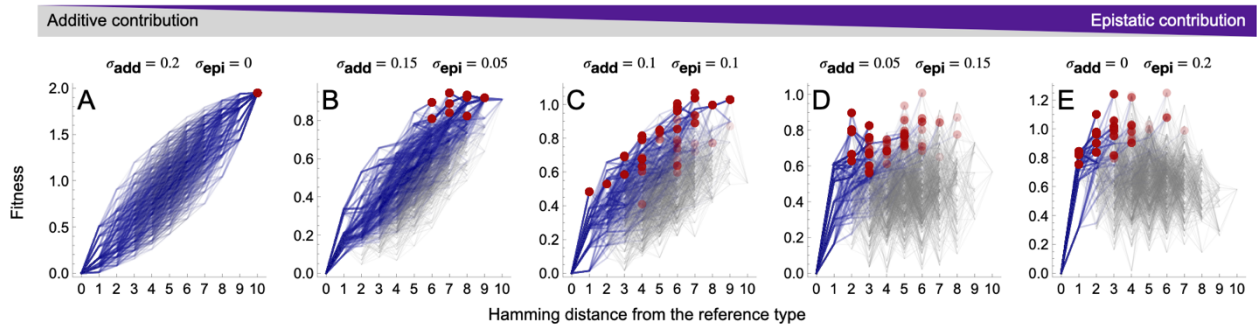

| F | Number of fitness peaks in the landscape                                            |      |      |      |      |
|---|-------------------------------------------------------------------------------------|------|------|------|------|
|   | 1                                                                                   | 9    | 49   | 90   | 101  |
|   | Number of fitness peaks that were reached in 1000 simulations                       |      |      |      |      |
|   | 1                                                                                   | 9    | 44   | 54   | 35   |
|   | Number of unique mutational steps that were taken in 1000 simulations               |      |      |      |      |
|   | 3464                                                                                | 2374 | 1271 | 409  | 167  |
|   | Average Hamming distance between any two evolutionary endpoints in 1000 simulations |      |      |      |      |
|   | 0                                                                                   | 2.42 | 4.45 | 3.78 | 3.22 |
